# Supplementary material for: Backcasting COVID-19: A Physics-Informed Estimate for Early Case Incidence
Source: arXiv:2202.00507 source file (2022-01-31)
Supplement: Supplementary file 1 [file AppendixC.tex]

The capture-recapture method was introduced in \cite{bohning2020} and is replicated here for
completion. 
Denote by $C(t)$ the cumulative number of infections at day $t$ and with $D(t)$, the  cumulative 
number of deaths at day $t$.
Then the new cases and new deaths, respectively, at day $t$ are given by 
\[
\Delta C(t) = C(t)-C(t-1)~~\mbox{and}~~ \Delta D(t) = D(t)-D(t-1).
\]
Assume that the total population is sampled on a daily basis in order to detect infected individuals.
The capture-recapture method, as the name suggests, allows for the same individual to be captured, 
namely identified as infected more than one time. Now, let $n$ denote the number of times an 
individual is captured and let $1-p$ denote the probability of identifying an individual.
It then follows, using the geometric distribution, that the probability $P_n$ of identifying an 
infected $n$ times equals
\[
P_n = p (1-p)^n,
\]
from which the probability of missing an infected individual is equal to
\[
P_0 = \frac{P_1^2}{P_2}.
\]
The next step in the method is to replace these theoretical probabilities with the 
frequencies of those identified just once $f_1$ and just twice $f_2$, respectively. 

As explained in \cite{bohning2020}, using COVID-19 data it follows that an estimate for the number of hidden infections is 
\[
\frac{[\Delta C(t)]^2}{\Delta C(t-1) -\Delta D(t)},
\]
since on day $t$ there are $\Delta C(t)$ new infections (interpreted as $f_1$) and those still 
infected on day $t$ that were also identified on day $t-1$ and are not deceased 
$\Delta C(t-1) -\Delta D(t)$ (interpreted as $f_2$). 
Furthermore, the equation for the variance is defined  in \cite{bohning2020}
as 
\[
\frac{[\Delta C(t)]^4}{[1+\Delta C(t-1) -\Delta D(t)]^3} +
\frac{4 [\Delta C(t)]^3}{[1+\Delta C(t-1) -\Delta D(t)]^2} +
\frac{[\Delta C(t)]^2}{[1+\Delta C(t-1) -\Delta D(t)]},
\]
which is used as an uncertainty measure.

\textcolor{red}{GAK: appendix to be removed once everybody has checked}
